# Supplementary material for: SmartTrack: Efficient Predictive Race Detection
Source: arXiv:1905.00494 source file (2020-04-09)
Supplement: Supplementary file 1 [file supplementary.pdf]

## A Predictable Race Coverage

Table 7 reports how many races each analysis finds. For each cell, the second value (in parentheses) is total dynamic races reported, and the first value is *statically distinct* races. Two dynamic races detected at the same static program location are the same statically unique race.

Although the analyses get progressively more powerful from top to bottom (e.g., every DC-race is a WDC-race), this relationship does not always hold empirically for two reasons. First, run-to-run variation naturally affects repeatability. Table 12 provides 95% confidence intervals for these results, showing that many of the differences involve overlapping confidence intervals. Second, analyses have different performance characteristics that may affect the evaluated program's memory interleaving behavior, leading to different races occurring.

For each relation, the different algorithms (*Unopt*-, *FTO*-, *ST*-) often report comparable race counts, but sometimes the counts differ significantly, especially the counts of statically distinct races. These differences occur for the above reasons plus a third reason: the different optimization levels have different behavior after they detect the first race, because they use different metadata (e.g., epochs vs. vector clocks) to order the race and detect future races (Section 5.1). These differences impact statically unique races the most.

For each relation, the differences between the *algorithms* (*Unopt*-, *FTO*-, *ST*-) are not a reflection of race detection effectiveness. The extra races detected by one algorithm, even if statistically significant, are likely to be related to each other, e.g., involving accesses to the same data structure as other reported races or being dependent on other reported races, and thus not be of much use to programmers. Rather, the race differences serve to show that the proposed optimizations and our implementations of them lead to reasonable race detection results.

Relatedly, the differences across relations do not serve mainly to demonstrate the effectiveness of weaker predictive analyses. Prior work has shown the relative effectiveness of WCP and DC analyses by performing HB, WCP, and DC analyses on the same observed trace [30, 53]. (Our results often report many more races, especially dynamic races, than prior work's results that used the RoadRunner Vindicator implementation and the DaCapo benchmarks [53]. These differences occur because the prior work used default RoadRunner behavior that stops performing analysis for a field after 100 dynamic races detected on the field, whereas our analyses disable that behavior.)

The results do show that despite using a weaker relation than DC analysis, WDC analysis does not on average report more races than DC analysis, which suggests that WDC analysis's optimization does not lead to false races in practice. In separate experiments with the *Unopt*-{DC, WDC} w/G analyses, *VINDICATERACE* successfully vindicates every DC- and WDC-race detected across 10 trials.

## B Results with Confidence Intervals

Tables 8, 9, 10, 11, and 12 show the same results as Tables 3, 5, 6, and 7, respectively, but with 95% confidence intervals.

## C SmartTrack Run-Time Characteristics

Table 13 reports frequencies of each FTO case for SmartTrack-WDC analysis, averaged over the 10 trials. The *Total* column counts the *non-same-epoch* reads and writes, i.e., all events except accesses that take [READ SAME EPOCH], [SHARED SAME EPOCH], or [WRITE SAME EPOCH] cases. Each value in the remaining columns represents, for a specific read or write case, the percentage of the total non-same-epoch reads or writes, respectively.

|     | Unopt-      | FTO-        | ST-         | Unopt-      | FTO-        | ST-         | Unopt-      | FTO-        | ST-         | Unopt-       | FTO-        | ST-          |
|-----|-------------|-------------|-------------|-------------|-------------|-------------|-------------|-------------|-------------|--------------|-------------|--------------|
| HB  | 6 (136,275) | 6 (103,752) | N/A         | 12 (40,548) | 17 (27,838) | N/A         | 3 (4)       | 3 (4)       | N/A         | 1 (1)        | 1 (1)       | N/A          |
| WCP | 5 (118,726) | 6 (103,717) | 6 (103,095) | 13 (40,924) | 10 (39,723) | 12 (34,004) | 3 (4)       | 3 (3)       | 3 (4)       | 1 (1)        | 1 (1)       | 1 (1)        |
| DC  | 6 (216,055) | 6 (104,288) | 7 (105,173) | 13 (41,295) | 12 (39,821) | 14 (35,613) | 4 (6)       | 1 (2)       | 3 (4)       | 1 (1)        | 1 (1)       | 1 (1)        |
| WDC | 6 (255,123) | 6 (105,449) | 6 (105,695) | 13 (41,439) | 12 (39,871) | 13 (32,108) | 3 (5)       | 2 (3)       | 3 (4)       | 1 (1)        | 1 (1)       | 1 (1)        |
|     | avrora      |             |             | h2          |             |             | jython      |             |             | luindex      |             |              |
|     | Unopt-      | FTO-        | ST-         | Unopt-      | FTO-        | ST-         | Unopt-      | FTO-        | ST-         | Unopt-       | FTO-        | ST-          |
| HB  | 3 (20)      | 7 (38)      | N/A         | 3 (7)       | 6 (12)      | N/A         | 60 (12,815) | 70 (13,086) | N/A         | 3 (17)       | 4 (17)      | N/A          |
| WCP | 4 (18)      | 7 (36)      | 7 (35)      | 3 (9)       | 3 (14)      | 3 (15)      | 56 (10,924) | 64 (13,537) | 68 (13,470) | 6 (239,437)  | 6 (234,441) | 7 (245,745)  |
| DC  | 8 (549)     | 7 (112)     | 7 (111)     | 3 (14)      | 5 (25)      | 5 (21)      | 97 (26,022) | 73 (12,933) | 75 (13,113) | 15 (416,002) | 8 (266,893) | 11 (288,608) |
| WDC | 7 (575)     | 7 (257)     | 7 (259)     | 3 (14)      | 7 (29)      | 5 (20)      | 91 (27,645) | 73 (12,866) | 71 (13,476) | 14 (405,776) | 8 (262,517) | 11 (287,563) |
|     | pmd         |             |             | sunflow     |             |             | tomcat      |             |             | xalan        |             |              |

**Table 7.** Average races reported by various analyses for each evaluated program (excluding batik and lusearch, for which all analyses report no races). In each cell, the first value is statically distinct races (i.e., distinct program locations) and the second value, in parentheses, is total dynamic races.

| Program  | Base<br>time | HB                            |                               |                               | Unopt-DC                    |                              | Unopt-WDC                    |                              |
|----------|--------------|-------------------------------|-------------------------------|-------------------------------|-----------------------------|------------------------------|------------------------------|------------------------------|
|          |              | RRFT2                         | FT2                           | FTO                           | w/ G                        | w/o G                        | w/ G                         | w/o G                        |
| avrora   | 2.4 s        | $7.2 \times \pm 0.13 \times$  | $4.6 \times \pm 0.38 \times$  | $4.6 \times \pm 0.24 \times$  | $28 \times \pm 1.2 \times$  | $24 \times \pm 1.4 \times$   | $27 \times \pm 3.4 \times$   | $23 \times \pm 1.5 \times$   |
| batik    | 2.8 s        | $4.2 \times \pm 0.053 \times$ | $4.2 \times \pm 0.064 \times$ | $4.1 \times \pm 0.068 \times$ | $12 \times \pm 0.21 \times$ | $11 \times \pm 0.13 \times$  | $12 \times \pm 0.30 \times$  | $11 \times \pm 0.14 \times$  |
| h2       | 5.2 s        | $9.5 \times \pm 0.58 \times$  | $8.9 \times \pm 0.25 \times$  | $8.7 \times \pm 0.21 \times$  | $82 \times \pm 9.3 \times$  | $74 \times \pm 3.7 \times$   | $79 \times \pm 6.3 \times$   | $78 \times \pm 8.9 \times$   |
| jython   | 4.1 s        | $8.4 \times \pm 0.23 \times$  | $8.9 \times \pm 0.33 \times$  | $8.8 \times \pm 0.31 \times$  | $36 \times \pm 1.5 \times$  | $33 \times \pm 4.6 \times$   | $33 \times \pm 1.8 \times$   | $27 \times \pm 1.1 \times$   |
| luindex  | 1.3 s        | $7.8 \times \pm 0.24 \times$  | $7.8 \times \pm 0.37 \times$  | $7.9 \times \pm 0.31 \times$  | $48 \times \pm 2.2 \times$  | $44 \times \pm 0.76 \times$  | $46 \times \pm 0.96 \times$  | $43 \times \pm 0.64 \times$  |
| lusearch | 1.6 s        | $7.8 \times \pm 0.35 \times$  | $7.9 \times \pm 0.39 \times$  | $7.8 \times \pm 0.42 \times$  | $27 \times \pm 7.2 \times$  | $23 \times \pm 0.96 \times$  | $24 \times \pm 1.3 \times$   | $29 \times \pm 9.6 \times$   |
| pmd      | 2.5 s        | $4.1 \times \pm 0.15 \times$  | $3.9 \times \pm 0.10 \times$  | $3.9 \times \pm 0.070 \times$ | $10 \times \pm 0.78 \times$ | $9.3 \times \pm 0.32 \times$ | $9.9 \times \pm 0.48 \times$ | $9.3 \times \pm 0.32 \times$ |
| sunflow  | 1.4 s        | $24 \times \pm 1.0 \times$    | $24 \times \pm 2.1 \times$    | $68 \times \pm 2.6 \times$    | $120 \times \pm 34 \times$  | $120 \times \pm 57 \times$   | $120 \times \pm 32 \times$   | $92 \times \pm 3.7 \times$   |
| tomcat   | 1.3 s        | $34 \times \pm 3.2 \times$    | $3.7 \times \pm 0.37 \times$  | $3.6 \times \pm 0.38 \times$  | $58 \times \pm 2.1 \times$  | $50 \times \pm 1.8 \times$   | $52 \times \pm 1.8 \times$   | $41 \times \pm 1.4 \times$   |
| xalan    | 2.0 s        | $5.3 \times \pm 0.62 \times$  | $5.3 \times \pm 0.69 \times$  | $5.3 \times \pm 0.65 \times$  | $61 \times \pm 7.2 \times$  | $43 \times \pm 4.5 \times$   | $56 \times \pm 6.3 \times$   | $40 \times \pm 5.5 \times$   |
| geomean  |              | $8.7 \times$                  | $6.7 \times$                  | $7.3 \times$                  | $37 \times$                 | $33 \times$                  | $35 \times$                  | $31 \times$                  |
| Run time |              |                               |                               |                               |                             |                              |                              |                              |

**Table 8.** Run-time performance for various FastTrack-based HB analyses and for unoptimized DC and WDC analyses, relative to uninstrumented execution, with 95% confidence intervals.

| Program      | Base<br>memory | HB                            |                               |                               | Unopt-DC                    |                             | Unopt-WDC                   |                             |
|--------------|----------------|-------------------------------|-------------------------------|-------------------------------|-----------------------------|-----------------------------|-----------------------------|-----------------------------|
|              |                | RRFT2                         | FT2                           | FTO                           | w/ G                        | w/o G                       | w/ G                        | w/o G                       |
| avrora       | 160 MB         | $18 \times \pm 3.5 \times$    | $4.6 \times \pm 0.21 \times$  | $4.7 \times \pm 0.12 \times$  | $70 \times \pm 2.1 \times$  | $41 \times \pm 1.7 \times$  | $70 \times \pm 2.0 \times$  | $37 \times \pm 1.6 \times$  |
| batik        | 220 MB         | $5.5 \times \pm 0.061 \times$ | $5.5 \times \pm 0.070 \times$ | $5.5 \times \pm 0.067 \times$ | $51 \times \pm 1.2 \times$  | $46 \times \pm 0.36 \times$ | $51 \times \pm 1.7 \times$  | $46 \times \pm 0.45 \times$ |
| h2           | 1,700 MB       | $3.2 \times \pm 0.091 \times$ | $3.3 \times \pm 0.089 \times$ | $3.2 \times \pm 0.097 \times$ | $56 \times \pm 3.8 \times$  | $58 \times \pm 2.5 \times$  | $56 \times \pm 3.1 \times$  | $56 \times \pm 2.6 \times$  |
| jython       | 750 MB         | $6.2 \times \pm 0.11 \times$  | $6.5 \times \pm 0.072 \times$ | $6.4 \times \pm 0.13 \times$  | $31 \times \pm 0.67 \times$ | $17 \times \pm 0.64 \times$ | $25 \times \pm 0.51 \times$ | $15 \times \pm 0.90 \times$ |
| luindex      | 120 MB         | $4.8 \times \pm 0.073 \times$ | $4.9 \times \pm 0.088 \times$ | $5.0 \times \pm 0.086 \times$ | $62 \times \pm 2.2 \times$  | $49 \times \pm 1.8 \times$  | $62 \times \pm 2.2 \times$  | $49 \times \pm 1.8 \times$  |
| lusearch     | 960 MB         | $15 \times \pm 2.7 \times$    | $15 \times \pm 2.8 \times$    | $15 \times \pm 2.6 \times$    | $22 \times \pm 4.1 \times$  | $20 \times \pm 3.3 \times$  | $21 \times \pm 4.1 \times$  | $19 \times \pm 3.3 \times$  |
| pmd          | 600 MB         | $2.3 \times \pm 0.060 \times$ | $2.3 \times \pm 0.061 \times$ | $2.3 \times \pm 0.066 \times$ | $12 \times \pm 0.31 \times$ | $11 \times \pm 0.32 \times$ | $12 \times \pm 0.33 \times$ | $11 \times \pm 0.52 \times$ |
| sunflow      | 610 MB         | $8.1 \times \pm 0.065 \times$ | $7.8 \times \pm 0.35 \times$  | $33 \times \pm 2.8 \times$    | $26 \times \pm 1.8 \times$  | $24 \times \pm 1.7 \times$  | $26 \times \pm 1.2 \times$  | $26 \times \pm 0.40 \times$ |
| tomcat       | 510 MB         | $51 \times \pm 5.6 \times$    | $3.3 \times \pm 0.043 \times$ | $3.1 \times \pm 0.14 \times$  | $24 \times \pm 4.3 \times$  | $20 \times \pm 3.7 \times$  | $22 \times \pm 4.0 \times$  | $17 \times \pm 3.1 \times$  |
| xalan        | 690 MB         | $6.5 \times \pm 0.051 \times$ | $6.5 \times \pm 0.053 \times$ | $6.1 \times \pm 0.056 \times$ | $60 \times \pm 0.88 \times$ | $41 \times \pm 1.6 \times$  | $58 \times \pm 1.3 \times$  | $41 \times \pm 2.2 \times$  |
| geomean      |                | $7.8 \times$                  | $5.2 \times$                  | $6.0 \times$                  | $36 \times$                 | $29 \times$                 | $35 \times$                 | $27 \times$                 |
| Memory usage |                |                               |                               |                               |                             |                             |                             |                             |

**Table 9.** Memory performance for various FastTrack-based HB analyses and for unoptimized DC and WDC analyses, relative to uninstrumented execution, with 95% confidence intervals.

|     | Unopt-                       | FTO-                          | ST-                           | Unopt-                       | FTO-                          | ST-                           | Unopt-                      | FTO-                         | ST-                          |
|-----|------------------------------|-------------------------------|-------------------------------|------------------------------|-------------------------------|-------------------------------|-----------------------------|------------------------------|------------------------------|
| HB  | $22 \times \pm 1.5 \times$   | $4.6 \times \pm 0.24 \times$  | N/A                           | $8.2 \times \pm 0.12 \times$ | $4.1 \times \pm 0.068 \times$ | N/A                           | $41 \times \pm 11 \times$   | $8.7 \times \pm 0.21 \times$ | N/A                          |
| WCP | $28 \times \pm 1.1 \times$   | $8.8 \times \pm 0.24 \times$  | $6.7 \times \pm 0.29 \times$  | $12 \times \pm 0.13 \times$  | $7.0 \times \pm 0.097 \times$ | $4.8 \times \pm 0.037 \times$ | $82 \times \pm 4.8 \times$  | $55 \times \pm 4.3 \times$   | $12 \times \pm 0.36 \times$  |
| DC  | $24 \times \pm 1.4 \times$   | $9.5 \times \pm 0.27 \times$  | $7.3 \times \pm 0.29 \times$  | $11 \times \pm 0.13 \times$  | $6.9 \times \pm 0.074 \times$ | $4.8 \times \pm 0.072 \times$ | $74 \times \pm 3.7 \times$  | $55 \times \pm 5.4 \times$   | $12 \times \pm 0.57 \times$  |
| WDC | $23 \times \pm 1.5 \times$   | $6.8 \times \pm 0.26 \times$  | $5.3 \times \pm 0.26 \times$  | $11 \times \pm 0.14 \times$  | $6.9 \times \pm 0.098 \times$ | $4.7 \times \pm 0.085 \times$ | $78 \times \pm 8.9 \times$  | $55 \times \pm 6.3 \times$   | $11 \times \pm 0.28 \times$  |
|     | avrora                       |                               |                               | batik                        |                               |                               | h2                          |                              |                              |
|     | Unopt-                       | FTO-                          | ST-                           | Unopt-                       | FTO-                          | ST-                           | Unopt-                      | FTO-                         | ST-                          |
| HB  | $30 \times \pm 6.0 \times$   | $8.8 \times \pm 0.31 \times$  | N/A                           | $31 \times \pm 0.44 \times$  | $7.9 \times \pm 0.31 \times$  | N/A                           | $20 \times \pm 1.4 \times$  | $7.8 \times \pm 0.42 \times$ | N/A                          |
| WCP | $38 \times \pm 1.3 \times$   | $11 \times \pm 0.33 \times$   | $12 \times \pm 0.50 \times$   | $51 \times \pm 0.62 \times$  | $23 \times \pm 0.69 \times$   | $9.2 \times \pm 0.34 \times$  | $27 \times \pm 1.3 \times$  | $9.9 \times \pm 0.46 \times$ | $9.2 \times \pm 0.50 \times$ |
| DC  | $33 \times \pm 4.6 \times$   | $11 \times \pm 0.51 \times$   | $12 \times \pm 0.60 \times$   | $44 \times \pm 0.76 \times$  | $23 \times \pm 0.63 \times$   | $9.0 \times \pm 0.31 \times$  | $23 \times \pm 0.96 \times$ | $9.8 \times \pm 0.54 \times$ | $9.4 \times \pm 0.41 \times$ |
| WDC | $27 \times \pm 1.1 \times$   | $9.1 \times \pm 0.29 \times$  | $9.6 \times \pm 0.30 \times$  | $43 \times \pm 0.64 \times$  | $22 \times \pm 0.68 \times$   | $8.9 \times \pm 0.41 \times$  | $29 \times \pm 9.6 \times$  | $9.1 \times \pm 0.43 \times$ | $8.7 \times \pm 0.43 \times$ |
|     | jython                       |                               |                               | luindex                      |                               |                               | lusearch                    |                              |                              |
|     | Unopt-                       | FTO-                          | ST-                           | Unopt-                       | FTO-                          | ST-                           | Unopt-                      | FTO-                         | ST-                          |
| HB  | $9.5 \times \pm 0.75 \times$ | $3.9 \times \pm 0.070 \times$ | N/A                           | $90 \times \pm 2.3 \times$   | $68 \times \pm 2.6 \times$    | N/A                           | $42 \times \pm 1.5 \times$  | $3.6 \times \pm 0.38 \times$ | N/A                          |
| WCP | $11 \times \pm 0.55 \times$  | $4.0 \times \pm 0.073 \times$ | $4.6 \times \pm 0.055 \times$ | $170 \times \pm 52 \times$   | $74 \times \pm 2.2 \times$    | $27 \times \pm 1.1 \times$    | $55 \times \pm 1.9 \times$  | $5.5 \times \pm 0.56 \times$ | $5.5 \times \pm 0.59 \times$ |
| DC  | $9.3 \times \pm 0.32 \times$ | $4.0 \times \pm 0.059 \times$ | $4.5 \times \pm 0.10 \times$  | $120 \times \pm 57 \times$   | $72 \times \pm 3.9 \times$    | $27 \times \pm 1.5 \times$    | $50 \times \pm 1.8 \times$  | $6.0 \times \pm 0.66 \times$ | $6.1 \times \pm 0.65 \times$ |
| WDC | $9.3 \times \pm 0.32 \times$ | $4.0 \times \pm 0.067 \times$ | $4.5 \times \pm 0.086 \times$ | $92 \times \pm 3.7 \times$   | $71 \times \pm 2.8 \times$    | $27 \times \pm 1.3 \times$    | $41 \times \pm 1.4 \times$  | $4.0 \times \pm 0.50 \times$ | $4.3 \times \pm 0.57 \times$ |
|     | pmd                          |                               |                               | sunflow                      |                               |                               | tomcat                      |                              |                              |
|     | Unopt-                       | FTO-                          | ST-                           | Unopt-                       | FTO-                          | ST-                           | Unopt-                      | FTO-                         | ST-                          |
| HB  | $18 \times \pm 1.8 \times$   | $5.3 \times \pm 0.65 \times$  | N/A                           | $18 \times \pm 1.8 \times$   | $5.3 \times \pm 0.65 \times$  | N/A                           | $18 \times \pm 1.8 \times$  | $5.3 \times \pm 0.65 \times$ | N/A                          |
| WCP | $49 \times \pm 6.3 \times$   | $31 \times \pm 4.9 \times$    | $9.1 \times \pm 1.0 \times$   | $49 \times \pm 6.3 \times$   | $31 \times \pm 4.9 \times$    | $9.1 \times \pm 1.0 \times$   | $49 \times \pm 6.3 \times$  | $31 \times \pm 4.9 \times$   | $9.1 \times \pm 1.0 \times$  |
| DC  | $43 \times \pm 4.5 \times$   | $31 \times \pm 3.3 \times$    | $9.8 \times \pm 1.2 \times$   | $43 \times \pm 4.5 \times$   | $31 \times \pm 3.3 \times$    | $9.8 \times \pm 1.2 \times$   | $43 \times \pm 4.5 \times$  | $31 \times \pm 3.3 \times$   | $9.8 \times \pm 1.2 \times$  |
| WDC | $40 \times \pm 5.5 \times$   | $29 \times \pm 3.1 \times$    | $6.8 \times \pm 0.84 \times$  | $40 \times \pm 5.5 \times$   | $29 \times \pm 3.1 \times$    | $6.8 \times \pm 0.84 \times$  | $40 \times \pm 5.5 \times$  | $29 \times \pm 3.1 \times$   | $6.8 \times \pm 0.84 \times$ |
|     | xalan                        |                               |                               | xalan                        |                               |                               | xalan                       |                              |                              |

**Table 10.** Run time, relative to uninstrumented execution, of various analyses for each evaluated program with 95% confidence intervals.

|     | Unopt-                      | FTO-                          | ST-                          | Unopt-                      | FTO-                          | ST-                           | Unopt-                      | FTO-                          | ST-                          |
|-----|-----------------------------|-------------------------------|------------------------------|-----------------------------|-------------------------------|-------------------------------|-----------------------------|-------------------------------|------------------------------|
| HB  | $19 \times \pm 3.1 \times$  | $4.7 \times \pm 0.12 \times$  | N/A                          | $30 \times \pm 0.75 \times$ | $5.5 \times \pm 0.067 \times$ | N/A                           | $17 \times \pm 1.4 \times$  | $3.2 \times \pm 0.097 \times$ | N/A                          |
| WCP | $100 \times \pm 2.8 \times$ | $14 \times \pm 1.6 \times$    | $9.5 \times \pm 0.85 \times$ | $51 \times \pm 0.93 \times$ | $14 \times \pm 0.35 \times$   | $12 \times \pm 0.050 \times$  | $63 \times \pm 3.4 \times$  | $41 \times \pm 2.1 \times$    | $8.1 \times \pm 0.29 \times$ |
| DC  | $41 \times \pm 1.7 \times$  | $14 \times \pm 1.6 \times$    | $9.5 \times \pm 0.96 \times$ | $46 \times \pm 0.36 \times$ | $14 \times \pm 0.32 \times$   | $12 \times \pm 0.074 \times$  | $58 \times \pm 2.5 \times$  | $40 \times \pm 1.7 \times$    | $8.1 \times \pm 0.25 \times$ |
| WDC | $37 \times \pm 1.6 \times$  | $10 \times \pm 0.47 \times$   | $5.8 \times \pm 0.16 \times$ | $46 \times \pm 0.45 \times$ | $14 \times \pm 0.35 \times$   | $12 \times \pm 0.057 \times$  | $56 \times \pm 2.6 \times$  | $45 \times \pm 2.9 \times$    | $7.6 \times \pm 0.29 \times$ |
|     | avrora                      |                               |                              | batik                       |                               |                               | h2                          |                               |                              |
|     | Unopt-                      | FTO-                          | ST-                          | Unopt-                      | FTO-                          | ST-                           | Unopt-                      | FTO-                          | ST-                          |
| HB  | $20 \times \pm 1.6 \times$  | $6.4 \times \pm 0.13 \times$  | N/A                          | $34 \times \pm 1.2 \times$  | $5.0 \times \pm 0.086 \times$ | N/A                           | $19 \times \pm 3.3 \times$  | $15 \times \pm 2.6 \times$    | N/A                          |
| WCP | $20 \times \pm 1.0 \times$  | $12 \times \pm 0.54 \times$   | $13 \times \pm 0.62 \times$  | $68 \times \pm 2.5 \times$  | $23 \times \pm 0.28 \times$   | $8.9 \times \pm 0.48 \times$  | $29 \times \pm 5.1 \times$  | $16 \times \pm 3.1 \times$    | $17 \times \pm 2.7 \times$   |
| DC  | $17 \times \pm 0.64 \times$ | $13 \times \pm 0.35 \times$   | $13 \times \pm 0.87 \times$  | $49 \times \pm 1.8 \times$  | $23 \times \pm 0.30 \times$   | $10 \times \pm 0.61 \times$   | $20 \times \pm 3.3 \times$  | $16 \times \pm 2.9 \times$    | $17 \times \pm 3.2 \times$   |
| WDC | $15 \times \pm 0.90 \times$ | $8.8 \times \pm 0.16 \times$  | $10 \times \pm 0.56 \times$  | $49 \times \pm 1.8 \times$  | $23 \times \pm 0.37 \times$   | $8.1 \times \pm 0.076 \times$ | $19 \times \pm 3.3 \times$  | $16 \times \pm 3.0 \times$    | $16 \times \pm 2.9 \times$   |
|     | jython                      |                               |                              | luindex                     |                               |                               | lusearch                    |                               |                              |
|     | Unopt-                      | FTO-                          | ST-                          | Unopt-                      | FTO-                          | ST-                           | Unopt-                      | FTO-                          | ST-                          |
| HB  | $10 \times \pm 0.43 \times$ | $2.3 \times \pm 0.066 \times$ | N/A                          | $23 \times \pm 1.1 \times$  | $33 \times \pm 2.8 \times$    | N/A                           | $18 \times \pm 3.3 \times$  | $3.1 \times \pm 0.14 \times$  | N/A                          |
| WCP | $16 \times \pm 0.37 \times$ | $2.5 \times \pm 0.068 \times$ | $5.0 \times \pm 0.13 \times$ | $42 \times \pm 4.4 \times$  | $91 \times \pm 0.26 \times$   | $37 \times \pm 0.068 \times$  | $24 \times \pm 4.6 \times$  | $7.0 \times \pm 0.53 \times$  | $7.4 \times \pm 0.16 \times$ |
| DC  | $11 \times \pm 0.32 \times$ | $2.5 \times \pm 0.070 \times$ | $5.0 \times \pm 0.21 \times$ | $24 \times \pm 1.7 \times$  | $91 \times \pm 0.26 \times$   | $37 \times \pm 0.14 \times$   | $20 \times \pm 3.7 \times$  | $8.4 \times \pm 0.29 \times$  | $9.4 \times \pm 0.81 \times$ |
| WDC | $11 \times \pm 0.52 \times$ | $2.5 \times \pm 0.060 \times$ | $5.0 \times \pm 0.13 \times$ | $26 \times \pm 0.40 \times$ | $91 \times \pm 0.25 \times$   | $37 \times \pm 0.12 \times$   | $17 \times \pm 3.1 \times$  | $4.1 \times \pm 0.090 \times$ | $5.5 \times \pm 0.19 \times$ |
|     | pmd                         |                               |                              | sunflow                     |                               |                               | tomcat                      |                               |                              |
|     | Unopt-                      | FTO-                          | ST-                          | Unopt-                      | FTO-                          | ST-                           | Unopt-                      | FTO-                          | ST-                          |
| HB  | $23 \times \pm 0.76 \times$ | $6.1 \times \pm 0.056 \times$ | N/A                          | $23 \times \pm 0.76 \times$ | $6.1 \times \pm 0.056 \times$ | N/A                           | $23 \times \pm 0.76 \times$ | $6.1 \times \pm 0.056 \times$ | N/A                          |
| WCP | $48 \times \pm 2.2 \times$  | $31 \times \pm 2.5 \times$    | $17 \times \pm 0.63 \times$  | $48 \times \pm 2.2 \times$  | $31 \times \pm 2.5 \times$    | $17 \times \pm 0.63 \times$   | $48 \times \pm 2.2 \times$  | $31 \times \pm 2.5 \times$    | $17 \times \pm 0.63 \times$  |
| DC  | $41 \times \pm 1.6 \times$  | $31 \times \pm 1.4 \times$    | $17 \times \pm 0.71 \times$  | $41 \times \pm 1.6 \times$  | $31 \times \pm 1.4 \times$    | $17 \times \pm 0.71 \times$   | $41 \times \pm 1.6 \times$  | $31 \times \pm 1.4 \times$    | $17 \times \pm 0.71 \times$  |
| WDC | $41 \times \pm 2.2 \times$  | $29 \times \pm 2.1 \times$    | $14 \times \pm 0.71 \times$  | $41 \times \pm 2.2 \times$  | $29 \times \pm 2.1 \times$    | $14 \times \pm 0.71 \times$   | $41 \times \pm 2.2 \times$  | $29 \times \pm 2.1 \times$    | $14 \times \pm 0.71 \times$  |
|     | xalan                       |                               |                              | xalan                       |                               |                               | xalan                       |                               |                              |

**Table 11.** Memory usage, relative to uninstrumented execution, of various analyses for each evaluated program with 95% confidence intervals.

|     |                |                          |                         |                         |                          |                       |                       |                 |                 |  |
|-----|----------------|--------------------------|-------------------------|-------------------------|--------------------------|-----------------------|-----------------------|-----------------|-----------------|--|
|     |                | Unopt-                   | FTO-                    | ST-                     |                          |                       |                       |                 |                 |  |
|     | HB             | 6 ± 0 (136,275 ± 575)    | 6 ± 0 (103,752 ± 2,432) | N/A                     |                          |                       |                       |                 |                 |  |
|     | WCP            | 5 ± 0 (118,726 ± 859)    | 6 ± 0 (103,717 ± 2,950) | 6 ± 0 (103,095 ± 1,486) |                          |                       |                       |                 |                 |  |
|     | DC             | 6 ± 0 (216,055 ± 1,199)  | 6 ± 0 (104,288 ± 1,785) | 7 ± 1 (105,173 ± 2,083) |                          |                       |                       |                 |                 |  |
|     | WDC            | 6 ± 0 (255,123 ± 5,844)  | 6 ± 0 (105,449 ± 2,785) | 6 ± 0 (105,695 ± 2,636) |                          |                       |                       |                 |                 |  |
|     |                | avrora                   |                         |                         |                          |                       |                       |                 |                 |  |
|     | Relation       | Unopt-                   | FTO-                    | ST-                     |                          |                       |                       |                 |                 |  |
|     | HB             | 12 ± 1 (40,548 ± 105)    | 17 ± 2 (27,838 ± 3,008) | N/A                     |                          |                       |                       |                 |                 |  |
|     | WCP            | 13 ± 0 (40,924 ± 47)     | 10 ± 0 (39,723 ± 91)    | 12 ± 0 (34,004 ± 2,221) |                          |                       |                       |                 |                 |  |
|     | DC             | 13 ± 0 (41,295 ± 76)     | 12 ± 0 (39,821 ± 116)   | 14 ± 1 (35,613 ± 2,279) |                          |                       |                       |                 |                 |  |
|     | WDC            | 13 ± 0 (41,439 ± 70)     | 12 ± 0 (39,871 ± 62)    | 13 ± 0 (32,108 ± 2,922) |                          |                       |                       |                 |                 |  |
|     |                | h2                       |                         |                         |                          |                       |                       |                 |                 |  |
|     | Unopt-         | FTO-                     | ST-                     | Unopt-                  | FTO-                     | ST-                   | Unopt-                | FTO-            | ST-             |  |
| HB  | 3 ± 0 (4 ± 0)  | 3 ± 0 (4 ± 0)            | N/A                     | 1 ± 0 (1 ± 0)           | 1 ± 0 (1 ± 0)            | N/A                   | 3 ± 0 (20 ± 1)        | 7 ± 0 (38 ± 4)  | N/A             |  |
| WCP | 3 ± 0 (4 ± 0)  | 3 ± 0 (3 ± 0)            | 3 ± 0 (4 ± 0)           | 1 ± 0 (1 ± 0)           | 1 ± 0 (1 ± 0)            | 1 ± 0 (1 ± 0)         | 4 ± 0 (18 ± 3)        | 7 ± 0 (36 ± 3)  | 7 ± 0 (35 ± 4)  |  |
| DC  | 4 ± 1 (6 ± 1)  | 1 ± 1 (2 ± 1)            | 3 ± 1 (4 ± 1)           | 1 ± 0 (1 ± 0)           | 1 ± 0 (1 ± 0)            | 1 ± 0 (1 ± 0)         | 8 ± 0 (549 ± 46)      | 7 ± 0 (112 ± 6) | 7 ± 0 (111 ± 9) |  |
| WDC | 3 ± 1 (5 ± 1)  | 2 ± 0 (3 ± 1)            | 3 ± 0 (4 ± 1)           | 1 ± 0 (1 ± 0)           | 1 ± 0 (1 ± 0)            | 1 ± 0 (1 ± 0)         | 7 ± 0 (575 ± 34)      | 7 ± 0 (257 ± 2) | 7 ± 0 (259 ± 3) |  |
|     |                | jython                   |                         |                         | luindex                  |                       |                       | pmd             |                 |  |
|     | Unopt-         | FTO-                     | ST-                     |                         | Unopt-                   | FTO-                  | ST-                   |                 |                 |  |
| HB  | 3 ± 0 (7 ± 0)  | 6 ± 1 (12 ± 2)           | N/A                     |                         | 60 ± 12 (12,815 ± 2,512) | 70 ± 3 (13,086 ± 631) | N/A                   |                 |                 |  |
| WCP | 3 ± 0 (9 ± 1)  | 3 ± 0 (14 ± 1)           | 3 ± 0 (15 ± 0)          |                         | 56 ± 11 (10,924 ± 2,141) | 64 ± 1 (13,537 ± 140) | 68 ± 1 (13,470 ± 175) |                 |                 |  |
| DC  | 3 ± 0 (14 ± 0) | 5 ± 1 (25 ± 3)           | 5 ± 0 (21 ± 1)          |                         | 97 ± 19 (26,022 ± 5,100) | 73 ± 1 (12,933 ± 108) | 75 ± 2 (13,113 ± 84)  |                 |                 |  |
| WDC | 3 ± 0 (14 ± 0) | 7 ± 1 (29 ± 4)           | 5 ± 0 (20 ± 1)          |                         | 91 ± 18 (27,645 ± 5,419) | 73 ± 1 (12,866 ± 188) | 71 ± 1 (13,476 ± 551) |                 |                 |  |
|     |                | sunflow                  |                         |                         | tomcat                   |                       |                       |                 |                 |  |
|     |                | Unopt-                   | FTO-                    | ST-                     |                          |                       |                       |                 |                 |  |
|     | HB             | 3 ± 0 (17 ± 0)           | 4 ± 0 (17 ± 1)          | N/A                     |                          |                       |                       |                 |                 |  |
|     | WCP            | 6 ± 0 (239,437 ± 1,331)  | 6 ± 0 (234,441 ± 275)   | 7 ± 0 (245,745 ± 531)   |                          |                       |                       |                 |                 |  |
|     | DC             | 15 ± 0 (416,002 ± 3,449) | 8 ± 0 (266,893 ± 574)   | 11 ± 0 (288,608 ± 582)  |                          |                       |                       |                 |                 |  |
|     | WDC            | 14 ± 0 (405,776 ± 4,517) | 8 ± 1 (262,517 ± 695)   | 11 ± 0 (287,563 ± 558)  |                          |                       |                       |                 |                 |  |
|     |                | xalan                    |                         |                         |                          |                       |                       |                 |                 |  |

**Table 12.** Average races reported by various analyses for each evaluated program (excluding batik and lusearch, for which all analyses report no races). In each cell, the first value is statically distinct races (i.e., distinct program locations) and the second value, in parentheses, is total dynamic races with 95% confidence intervals.

|          | Event Type | Total  | Owned |         | Unowned  |         |         |
|----------|------------|--------|-------|---------|----------|---------|---------|
|          |            |        | Excl  | Shared  | Excl     | Share   | Shared  |
| avrora   | Read       | 94 M   | 42.3% | 53.9%   | 1.97%    | 1.01%   | 0.814%  |
|          | Write      | 44 M   | 98.2% | N/A     | 0.328%   | N/A     | 1.48%   |
| batik    | Read       | 3.2 M  | 100%  | —       | 0.00692% | <0.001% | —       |
|          | Write      | 2.4 M  | 100%  | N/A     | —        | N/A     | <0.001% |
| h2       | Read       | 250 M  | 83.6% | 7.49%   | 8.35%    | 0.185%  | 0.341%  |
|          | Write      | 46 M   | 99.1% | N/A     | 0.26%    | N/A     | 0.637%  |
| jython   | Read       | 110 M  | 95.3% | 4.72%   | <0.001%  | <0.001% | —       |
|          | Write      | 28 M   | 100%  | N/A     | <0.001%  | N/A     | <0.001% |
| luindex  | Read       | 27 M   | 100%  | <0.001% | <0.001%  | <0.001% | —       |
|          | Write      | 13 M   | 100%  | N/A     | <0.001%  | N/A     | <0.001% |
| lusearch | Read       | 110 M  | 96.1% | 3.93%   | <0.001%  | <0.001% | <0.001% |
|          | Write      | 28 M   | 100%  | N/A     | —        | N/A     | <0.001% |
| pmd      | Read       | 7.4 M  | 98%   | 1.61%   | 0.153%   | 0.117%  | 0.0761% |
|          | Write      | 0.49 M | 98.5% | N/A     | 0.00163% | N/A     | 1.5%    |
| sunflow  | Read       | 2.5 M  | 4.03% | 70.2%   | 5.8%     | 3.24%   | 16.7%   |
|          | Write      | 0.96 M | 100%  | N/A     | <0.001%  | N/A     | 0.0163% |
| tomcat   | Read       | 5.7 M  | 56.1% | 27.5%   | 15.9%    | 0.274%  | 0.199%  |
|          | Write      | 4.5 M  | 69.4% | N/A     | 30.3%    | N/A     | 0.295%  |
| xalan    | Read       | 190 M  | 82.8% | 17.2%   | 0.042%   | 0.0189% | 0.0159% |
|          | Write      | 40 M   | 90%   | N/A     | 9.96%    | N/A     | 0.0764% |

**Table 13.** Frequencies of non-same-epoch reads and writes for SmartTrack-WDC, for each evaluated program.
